# Supplementary material for: Analysis of Aggregated Functional Data from Mixed Populations with Application to Energy Consumption
Source: arXiv:1402.1740 ancillary file (2014-02-07)
Supplement: Supplementary file 1 [file supplementary.pdf]

# Analysis of Aggregrated Functional Data from Mixed Populations with Application to Energy Consumption

Supplementary Material

Lenzi, A., de Souza, C. P. E., Dias, R., Garcia, N. and Heckman, N.

January 21, 2014

To study the effect of increasing the number of transformers as well as the number of replicates for Cases 1-4 (Section 6.1 of the paper) we conduct further simulation studies and present in this supplementary material the results for the following scenarios: (i) 5 transformers with 1, 5, 30 and 100 replicates and (ii) 50 transformers with 1 and 5 replicates.

Figures 1–12 present the pointwise mininum, maximum, first and third quartiles of the 200 estimated typologies for Cases 1-4 under all the different scenarios described in the previous paragraph. As expected, the variability of the estimated typologies is reduced by increasing the number of transformers and/or the number of replicates. In addition, the bias in typology estimation is reduced by increasing the number of transformers. Perhaps surprisingly, this bias is not reduced by increasing the number of replicates. Thus, in cases where estimates have a large bias and a decreased variability, the estimated typologies concentrate around the wrong curve.

Figures 13–16 present the histograms of the estimates of $\sigma^2$, the variance of the white noise, for all the different simulation scenarios. In addition, Table 1 presents the empirical variance and bias of the estimates of $\sigma^2$. From the table, we observe that, in almost all cases, the variability and the magnitude of the bias in the estimation of $\sigma^2$ are reduced by increasing the number of transformers and/or replicates. The three exceptions are when there are 50 transformers and we compare having no replicates to having 5 replicates. In

Cases 2 and 4, the magnitude of the bias is larger for 5 replicates than for no replicates. In Case 2, the variance is also larger. For Cases 2 and 4, from Figures 14 and 16 we see that the distribution of estimates is more skewed when there are 5 replicates. We do not know what might cause the skewness, but we may not want to compare the bias and variance of a skewed distribution to those of a symmetric distribution.

As pointed out in Section 6.2 of the paper the estimation of the variance parameters of the consumer level energy consumption curves, $\sigma^2_{\gamma,1}$ and $\sigma^2_{\gamma,2}$ , caused some problems, particularly when we consider only one day of data per transformer. In this case, in many data sets, the estimates of $\sigma^2_{\gamma,1}$ and $\sigma^2_{\gamma,2}$ are equal to zero. The percentage of estimates equal to zero for all different simulation scenarios are presented in Table 2. For Cases 1-4 we observe that by increasing the number of replicates and/or transformers the problem of obtaining estimates of $\sigma^2_{\gamma,2}$ that are equal to zero is resolved or drastically reduced. Regarding the estimation of $\sigma^2_{\gamma,1}$ the same is true only for Cases 1-2. For Case 4 the problem in the estimation of $\sigma^2_{\gamma,1}$ is reduced only for the scenario with 50 transformers and 5 replicates. Case 3 is the most challenging one as increasing the number of transformers and/or replicates does not reduce the number of zero estimates of $\sigma^2_{\gamma,1}$ to an acceptable level. From Table 2, we also observe that increasing the number of replicates or the number of transformers does seem to always reduce variance and does in most instances reduce bias.

Tables 3 and 4 present the simulated distribution of $\hat{M}_1$, the estimated number of consumers of class $c = 1$ (residential), for transformers $i = 1, \ldots, 5$ for simulations considering 5 and 50 transformers with 1 and 5 replicates. Table 3 presents the results for simulations with balanced $M$'s (Cases 1 and 3) and Table 4 the results for unbalanced $M$'s (Cases 2 and 4). The results of these tables are described in the body of the paper in Section 6.2. When considering increasing the number of replicates (tables not presented here), we found that the bias of the estimates typically did not decrease when we increased the number of replicates, but the variability did decrease.

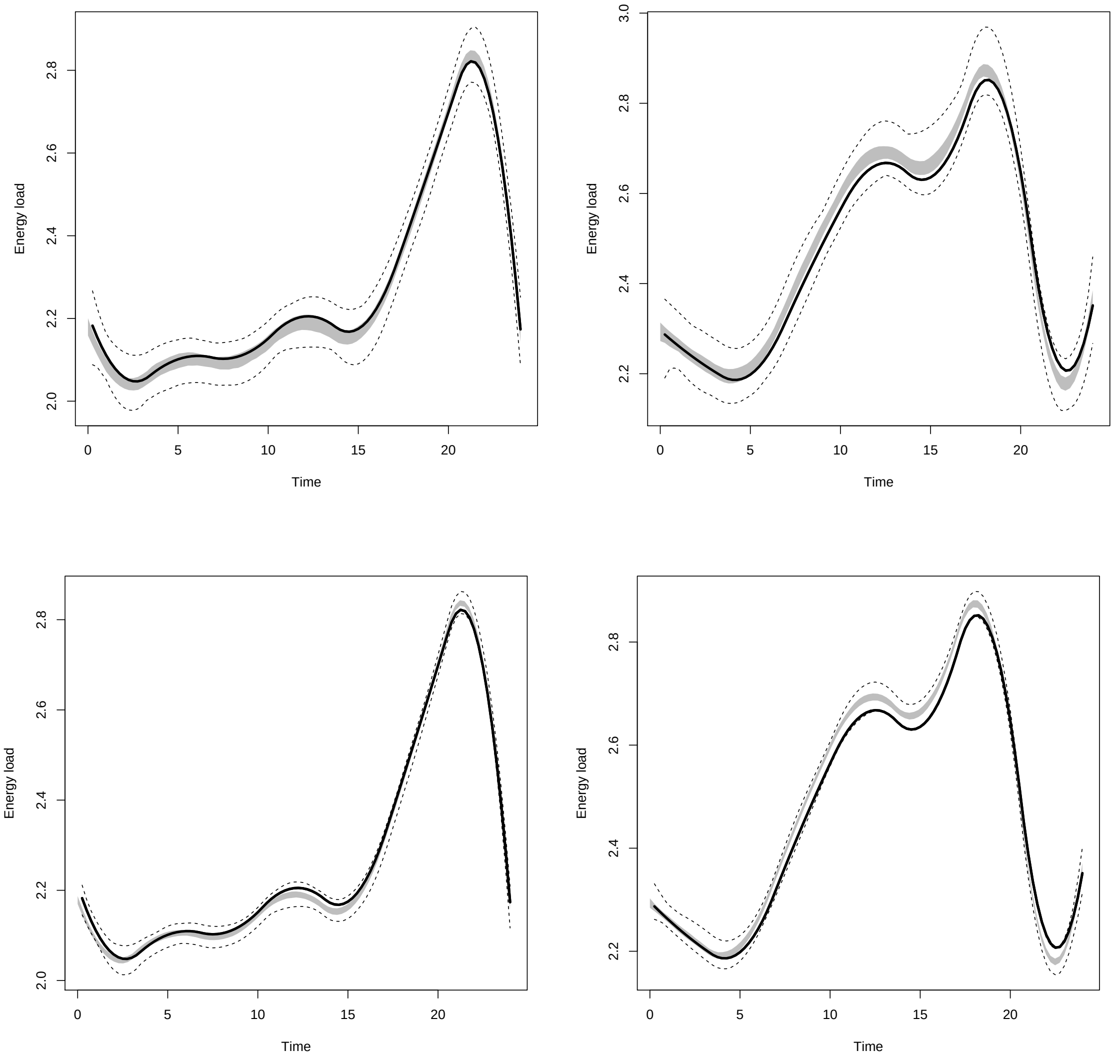


Figure 1: Case 1 ($\alpha_1$ *and* $\alpha_2$ *are of the same scale and the* $M$*'s are balanced*) - data generated with 5 transformers): pointwise minimum, maximum, first and third quartiles of the 200 estimated typologies for classes $c = 1$ residential (left column) and $c = 2$ commercial (right column) without replicates (top row) and with 5 replicates (bottom row). The solid curve is the true typology used to generate the data, the shaded gray area is the area between the first and third quartiles and the dashed lines are the minimum and maximum.

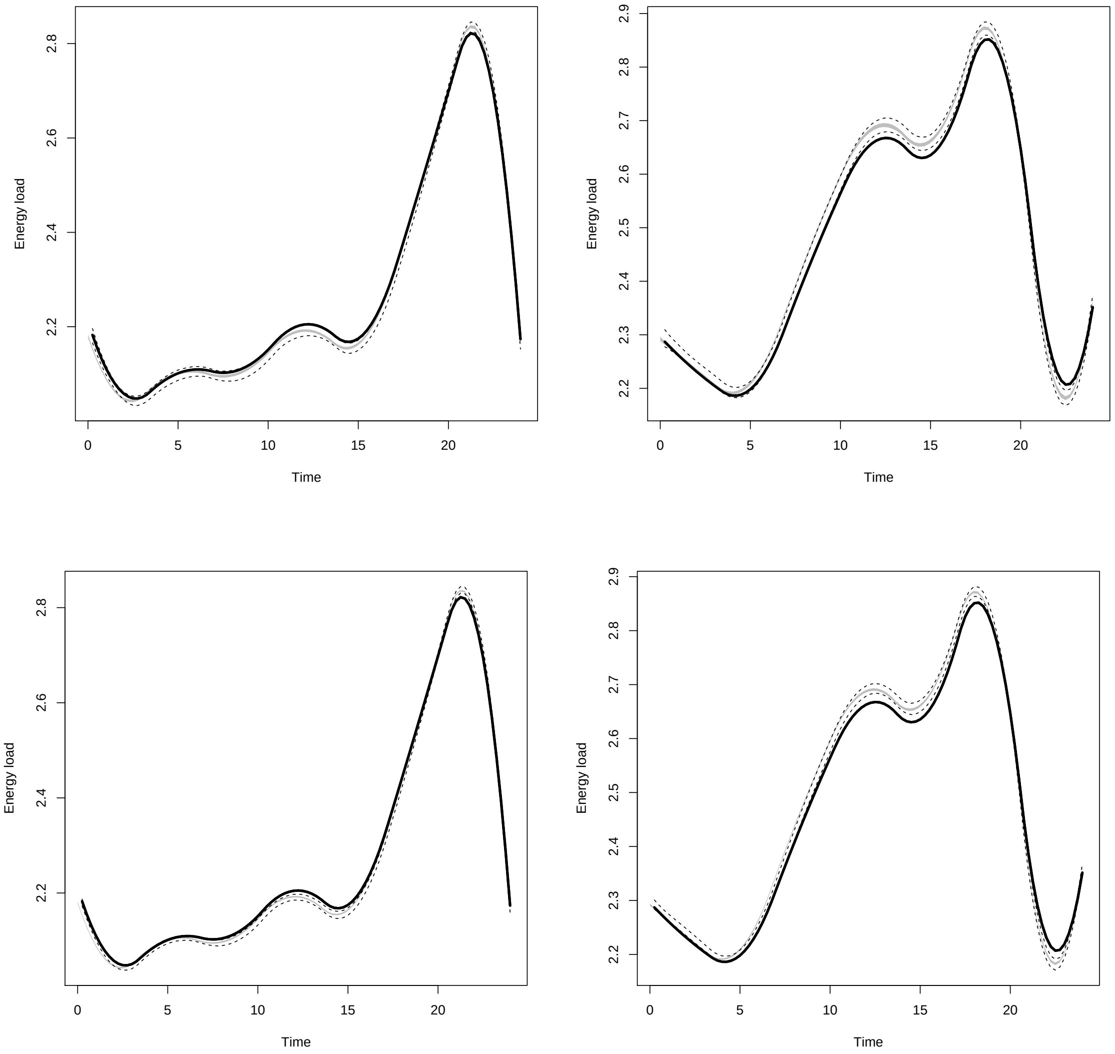


Figure 2: Case 1 ($\alpha_1$ *and* $\alpha_2$ *are of the same scale and the* $M$*'s are balanced*) - data generated with 5 transformers: pointwise minimum, maximum, first and third quartiles of the 200 estimated typologies for classes $c = 1$ residential (left column) and $c = 2$ commercial (right column) with 30 and 100 replicates (top and bottom rows, respectively) as in Figure 1.

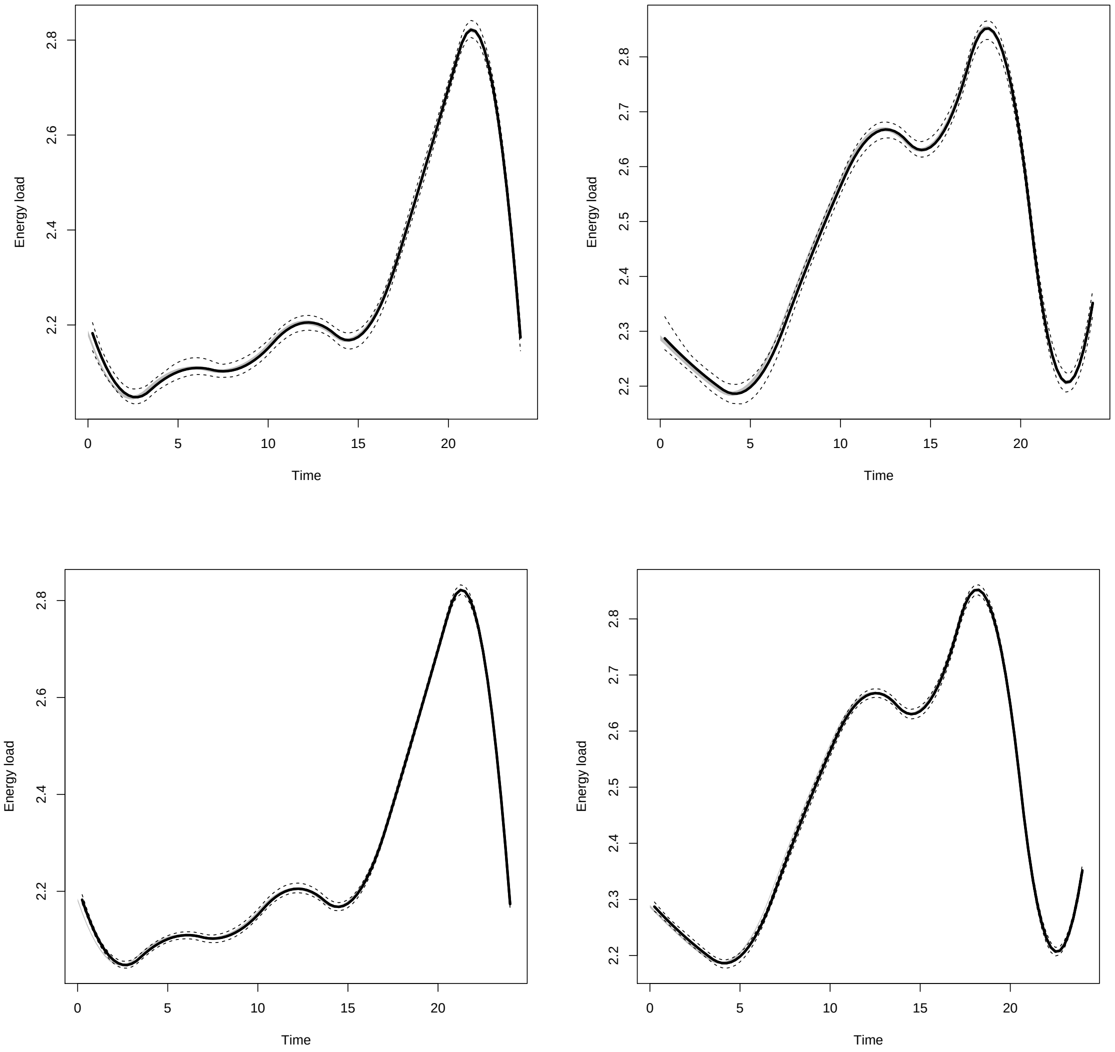


Figure 3: Case 1 ($\alpha_1$ *and* $\alpha_2$ *are of the same scale and the M's are balanced*) - data generated with 50 transformers: pointwise minimum, maximum, first and third quartiles of the 200 estimated typologies for residential (left column) and commercial (right column) without replicates (top row) and with 5 replicates (bottom row) as in Figure 1.

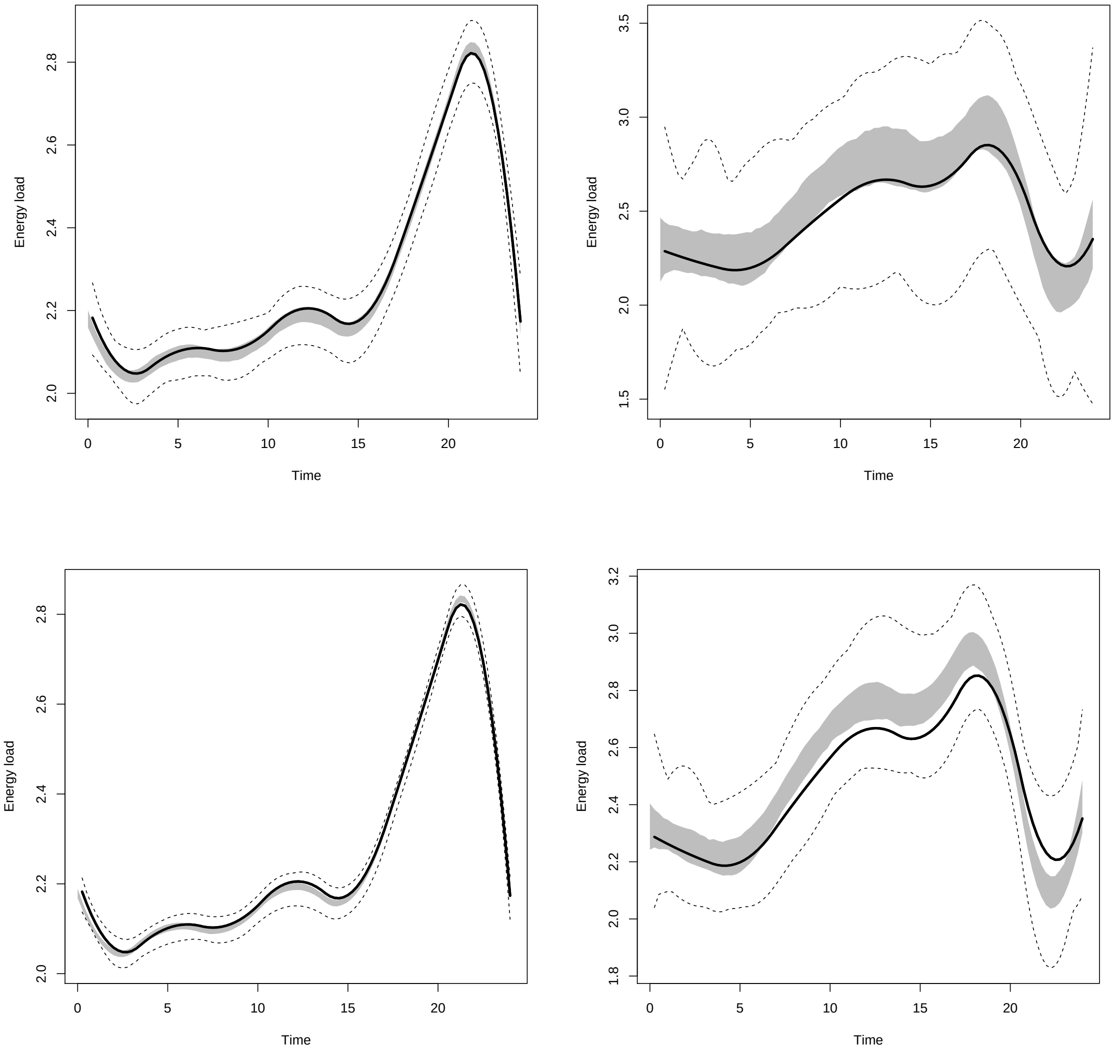


Figure 4: Case 2 (*$\alpha_1$ and $\alpha_2$ are of the same scale and the $M_1$'s are much bigger than the $M_2$'s*) - data generated with 5 transformers: pointwise minimum, maximum, first and third quartiles of the 200 estimated typologies for classes $c = 1$ residential (left column) and $c = 2$ commercial (right column) without replicates (top row) and with 5 replicates (bottom row) as in Figure 1.

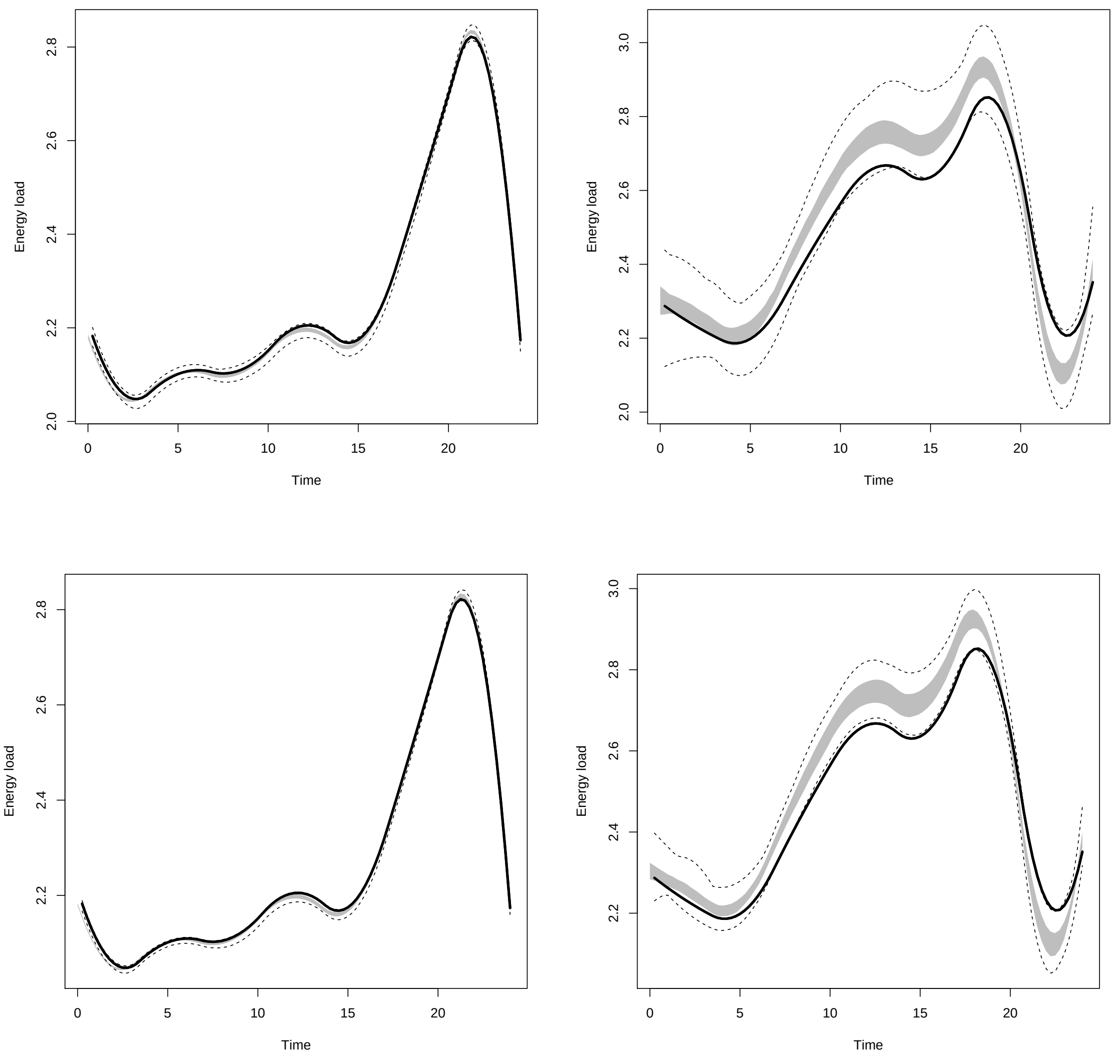


Figure 5: Case 2 ($\alpha_1$ *and* $\alpha_2$ *are of the same scale and the* $M_1$*'s are much bigger than the* $M_2$*'s*) - data generated with 5 transformers: pointwise minimum, maximum, first and third quartiles of the 200 estimated typologies for classes $c = 1$ residential (left column) and $c = 2$ commercial (right column) with 30 and 100 replicates (top and bottom rows, respectively) as in Figure 1.

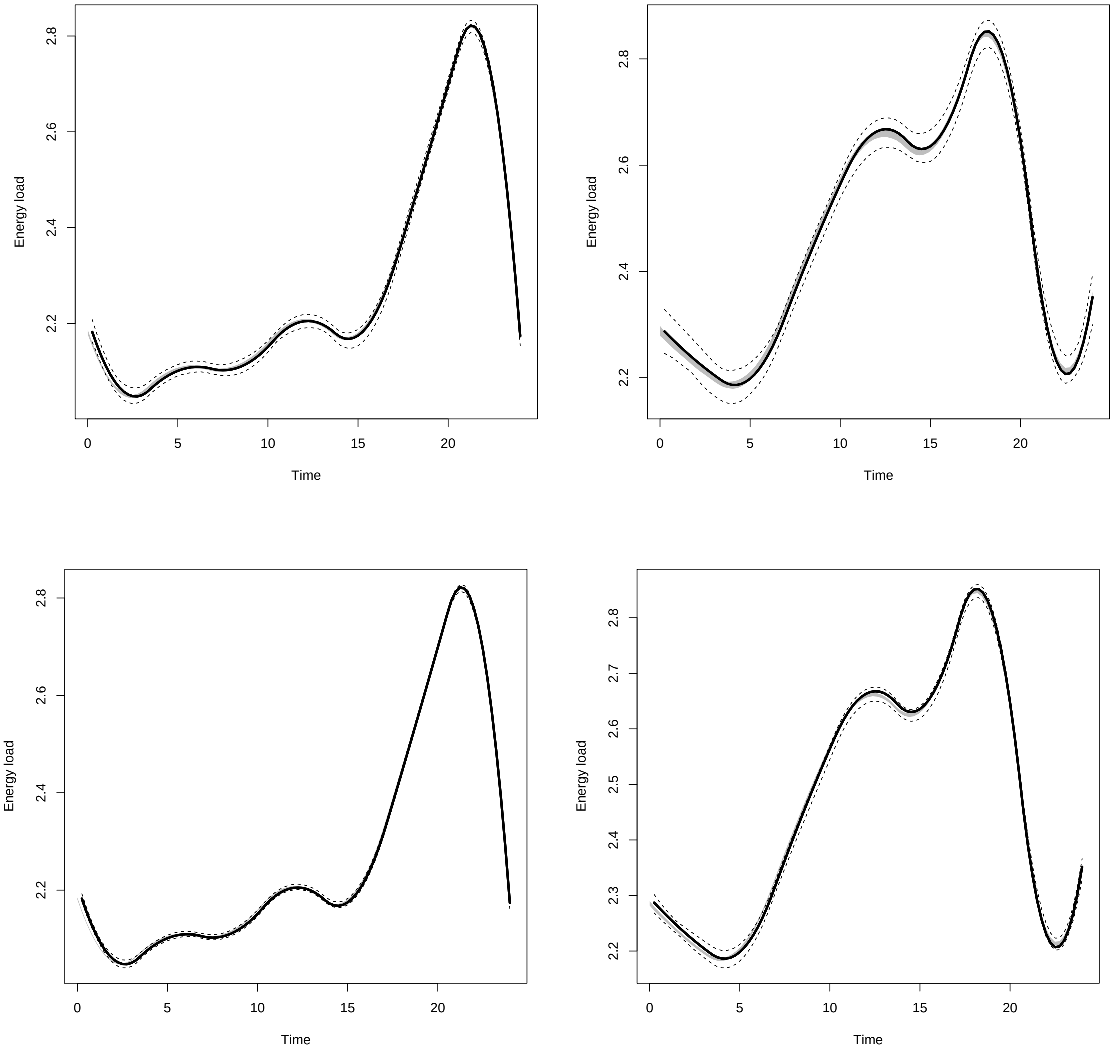


Figure 6: Case 2 (*$\alpha_1$ and $\alpha_2$ are of the same scale and the $M_1$'s are much bigger than the $M_2$'s*) - data generated with 50 transformers: pointwise minimum, maximum, first and third quartiles of the 200 estimated typologies for residential (left column) and commercial (right column) without replicates (top row) and with 5 replicates (bottom row) as in Figure 1.

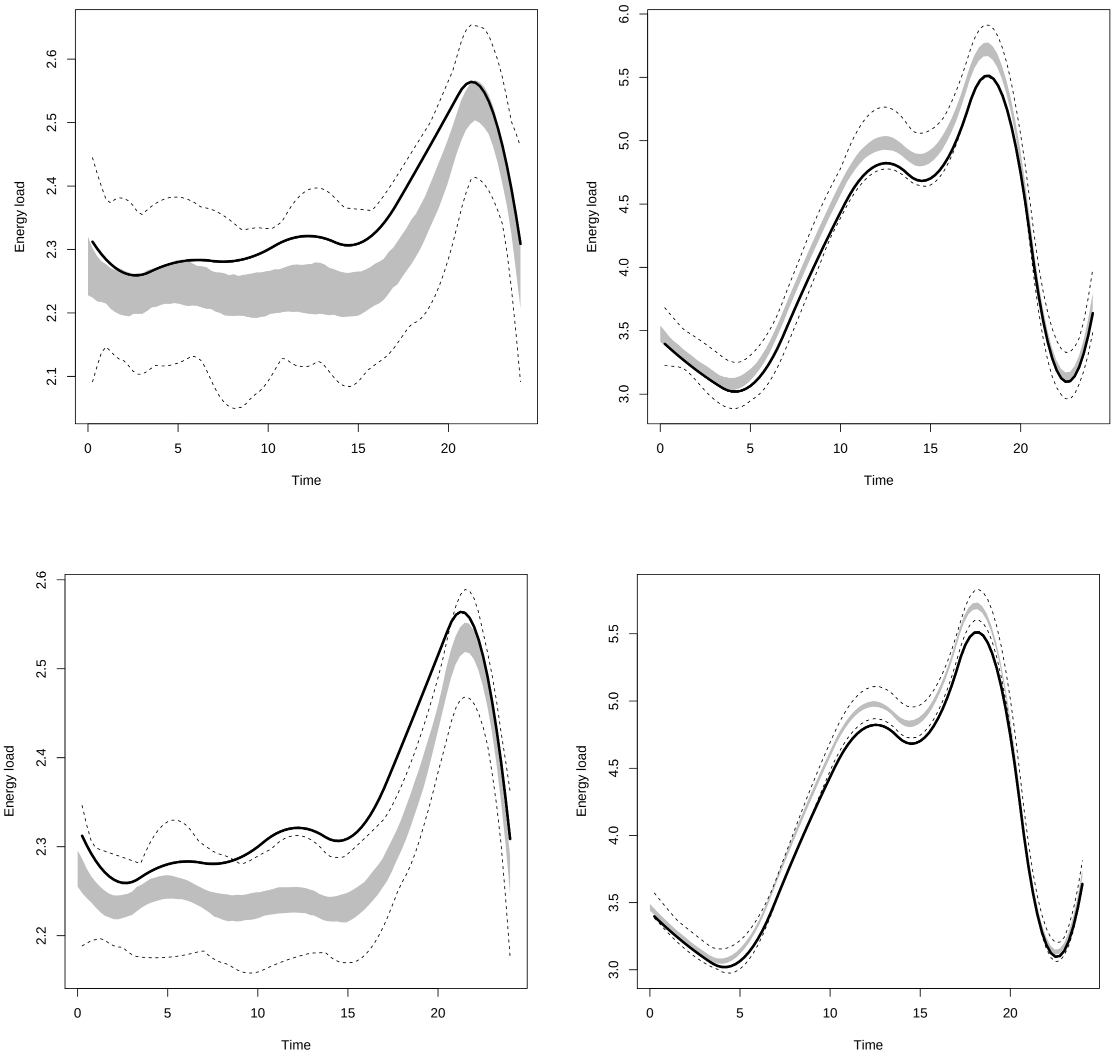


Figure 7: Case 3 ($\alpha_1$ *is much smaller than* $\alpha_2$ *and the M's are balanced*) - data generated with 5 transformers: pointwise minimum, maximum, first and third quartiles of the 200 estimated typologies for classes $c = 1$ residential (left column) and $c = 2$ commercial (right column) without replicates (top row) and with 5 replicates (bottom row) as in Figure 1.

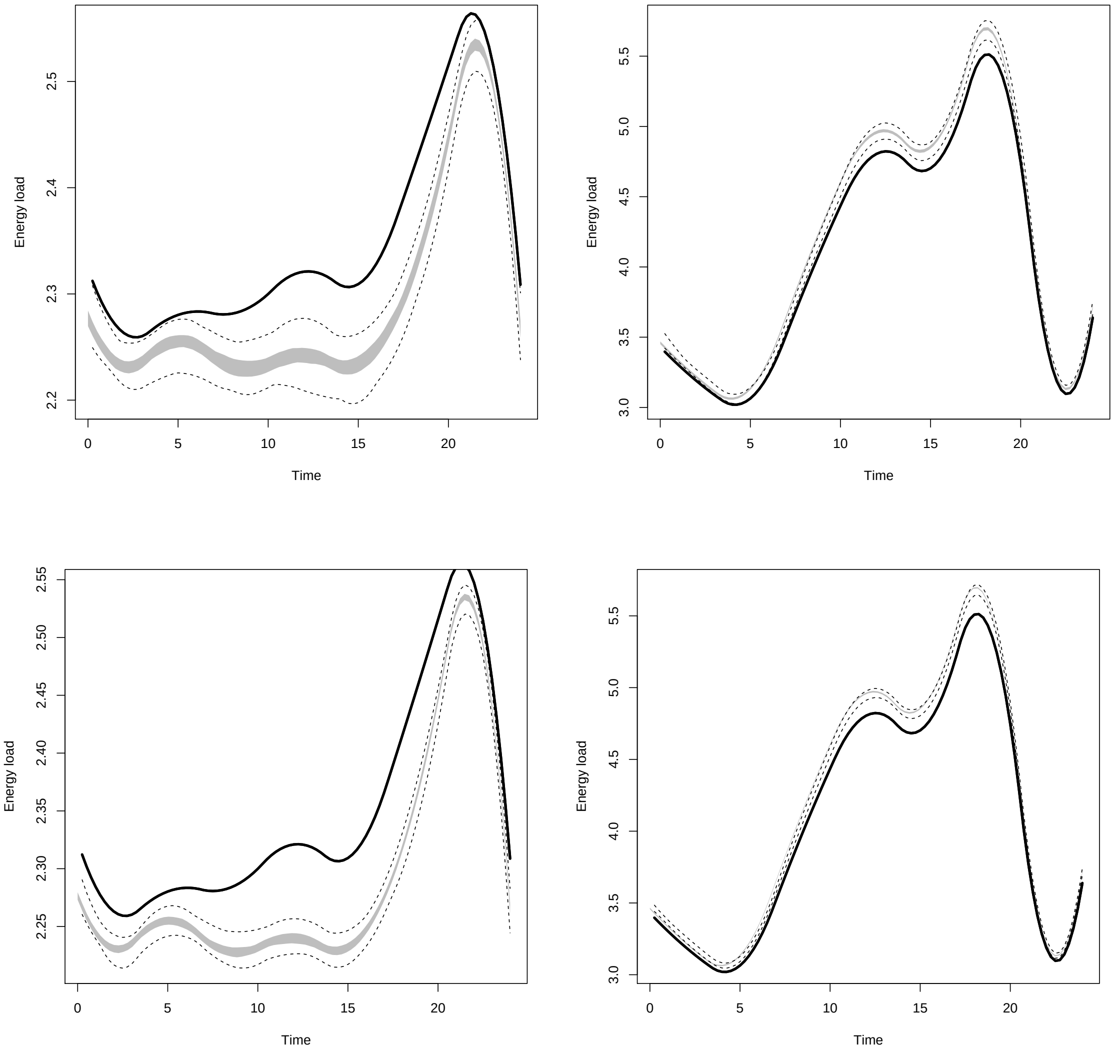


Figure 8: Case 3 ($\alpha_1$ *is much smaller than* $\alpha_2$ *and the* $M$*'s are balanced*) - data generated with 5 transformers: pointwise minimum, maximum, first and third quartiles of the 200 estimated typologies for classes $c = 1$ residential (left column) and $c = 2$ commercial (right column) with 30 and 100 replicates (top and bottom rows, respectively) as in Figure 1.

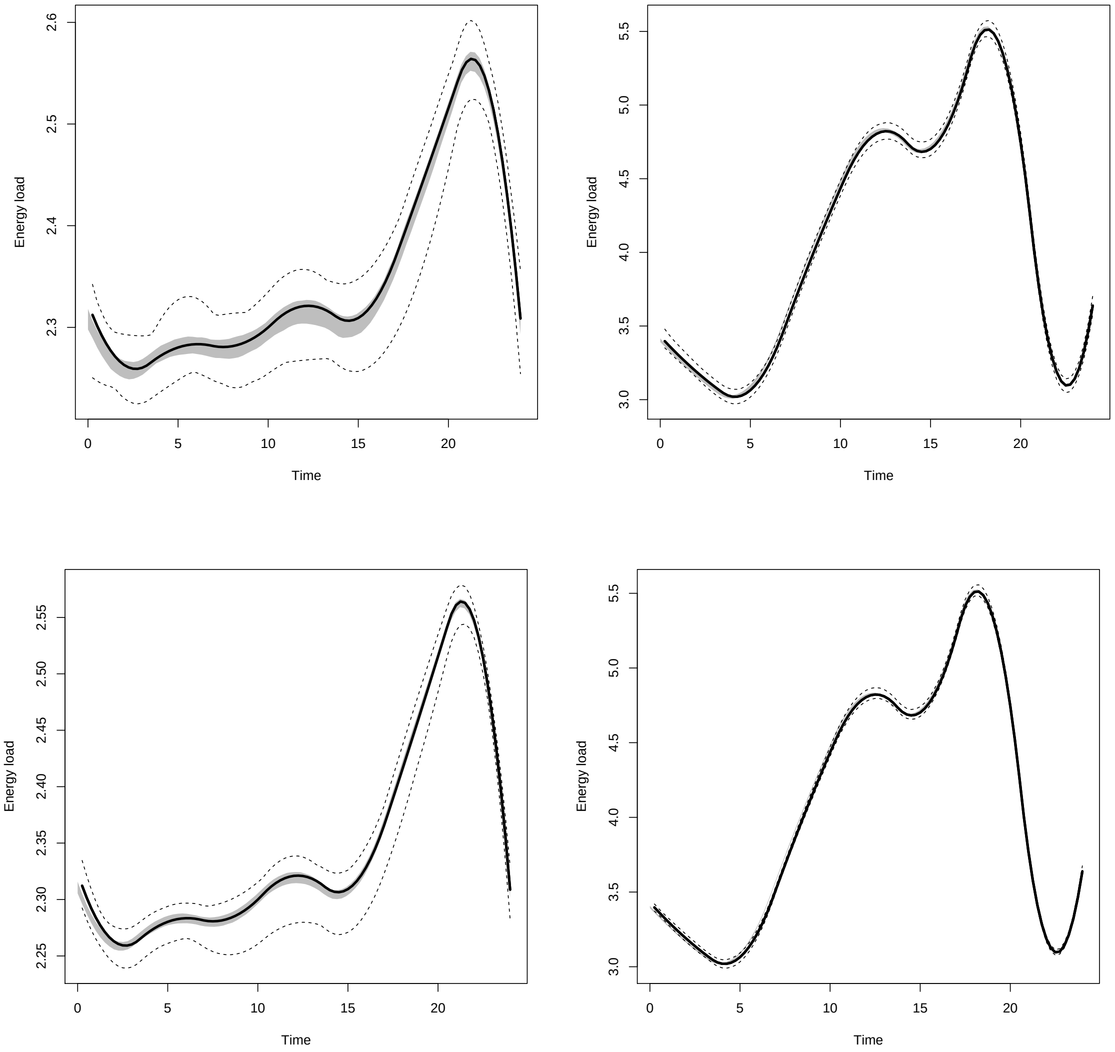


Figure 9: Case 3 ($\alpha_1$ *is much smaller than* $\alpha_2$ *and the M's are balanced*) - data generated with 50 transformers: pointwise minimum, maximum, first and third quartiles of the 200 estimated typologies for residential (left column) and commercial (right column) without replicates (top row) and with 5 replicates (bottom row) as in Figure 1.

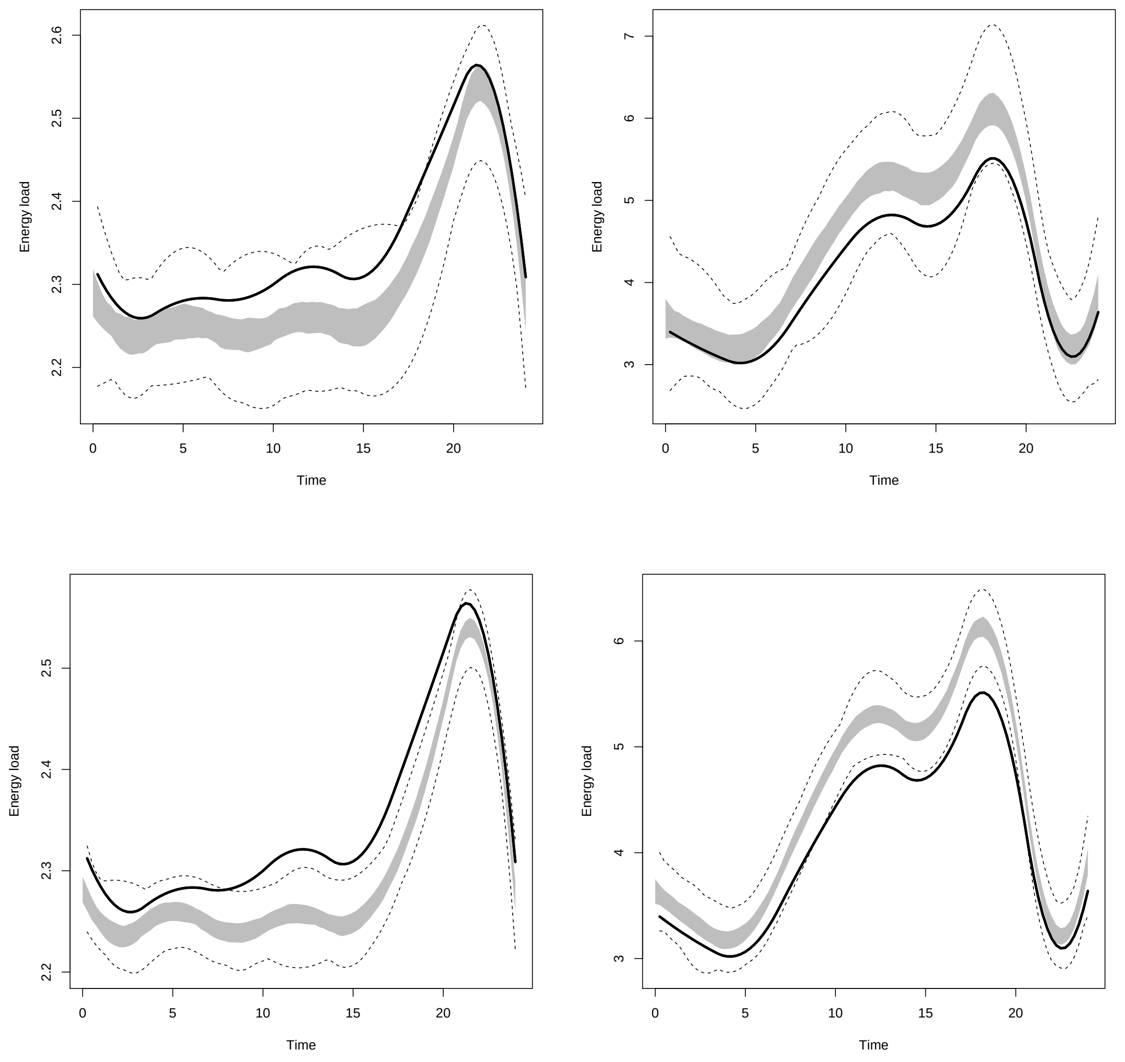


Figure 10: Case 4 ($\alpha_1$ *is much smaller than* $\alpha_2$ *and the* $M_1$*'s are much bigger than the* $M_2$*'s*) - data generated with 5 transformers: pointwise minimum, maximum, first and third quartiles of the 200 estimated typologies for classes $c = 1$ residential (left column) and $c = 2$ commercial (right column) without replicates (top row) and with 5 replicates (bottom row) as in Figure 1.

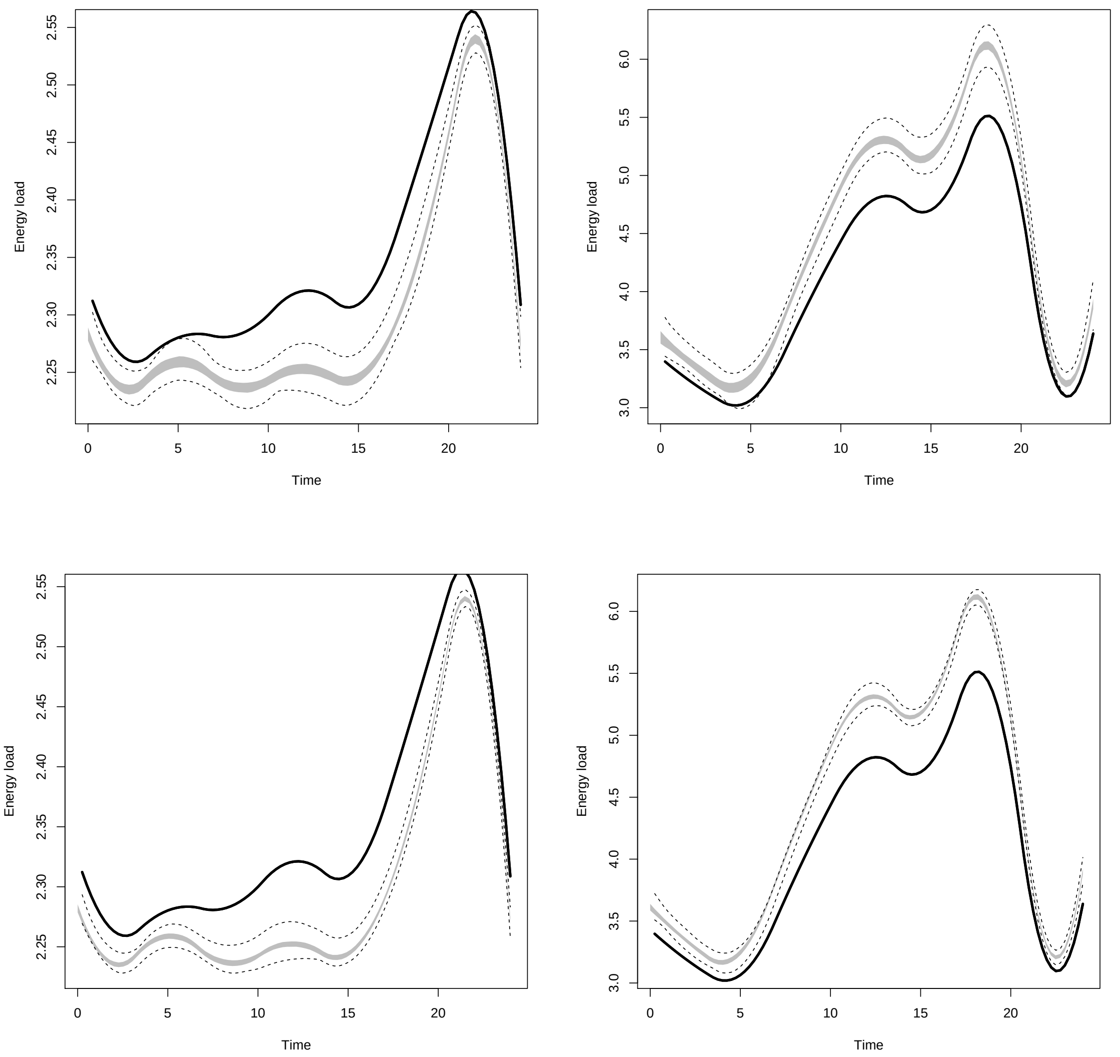


Figure 11: Case 4 ($\alpha_1$ *is much smaller than* $\alpha_2$ *and the* $M_1$*'s are much bigger than the* $M_2$*'s*) - data generated with 5 transformers: pointwise minimum, maximum, first and third quartiles of the 200 estimated typologies for classes $c = 1$ residential (left column) and $c = 2$ commercial (right column) with 30 and 100 replicates (top and bottom rows, respectively) as in Figure 1.

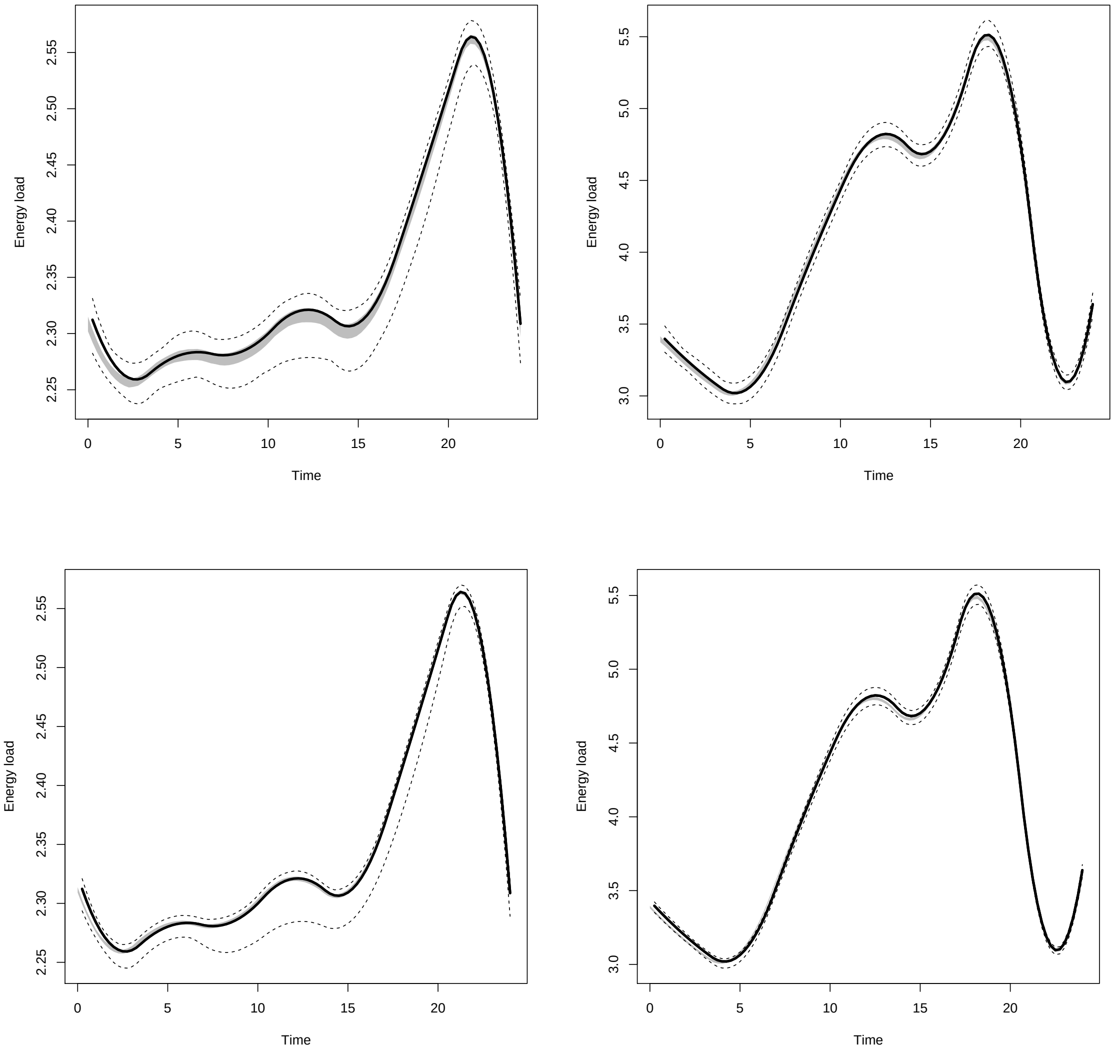


Figure 12: Case 4 ($\alpha_1$ *is much smaller than* $\alpha_2$ *and the* $M_1$*'s are much bigger than the* $M_2$*'s*) - data generated with 5 transformers: pointwise minimum, maximum, first and third quartiles of the 200 estimated typologies for residential (left column) and commercial (right column) without replicates (top row) and with 5 replicates (bottom row) as in Figure 1.

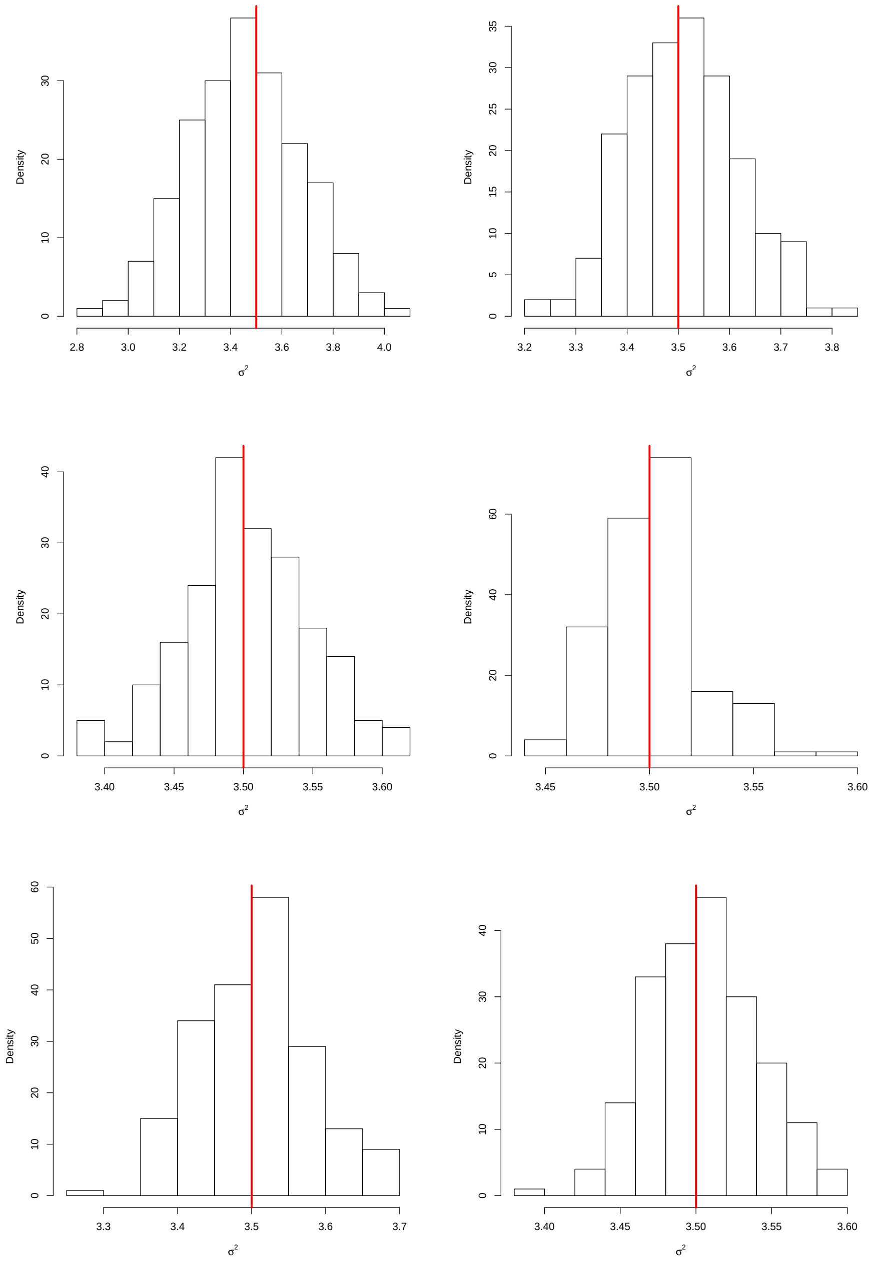


Figure 13: Case 1 ($\alpha_1$ *and* $\alpha_2$ *are of the same scale and the* $M$*'s are balanced*): histogram of the 200 estimates of the variance of the white noise. First row: data generated with 5 transformers without replicates (left) and with 5 replicates (right). Second row: data generated with 5 transformers with 30 (left) and 100 replicates (right). Third row: data generated with 50 transformers without replicates (left) and with 5 replicates (right). The vertical line represents the true value.

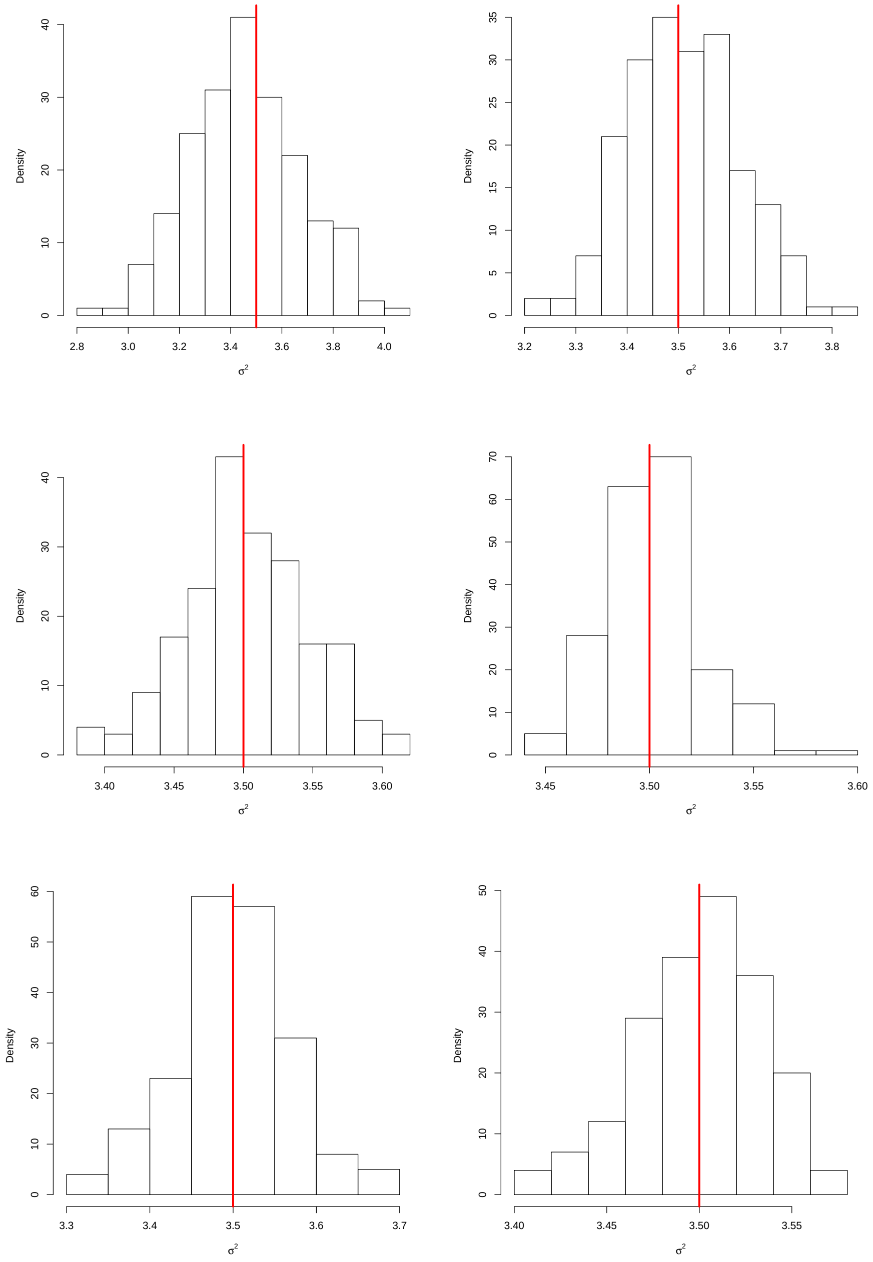


Figure 14: Case 2 ($\alpha_1$ *and* $\alpha_2$ *are of the same scale and the* $M_1$*'s are much bigger than the* $M_2$*'s*): histogram of the 200 estimates of the variance of the white noise as in Figure 13.

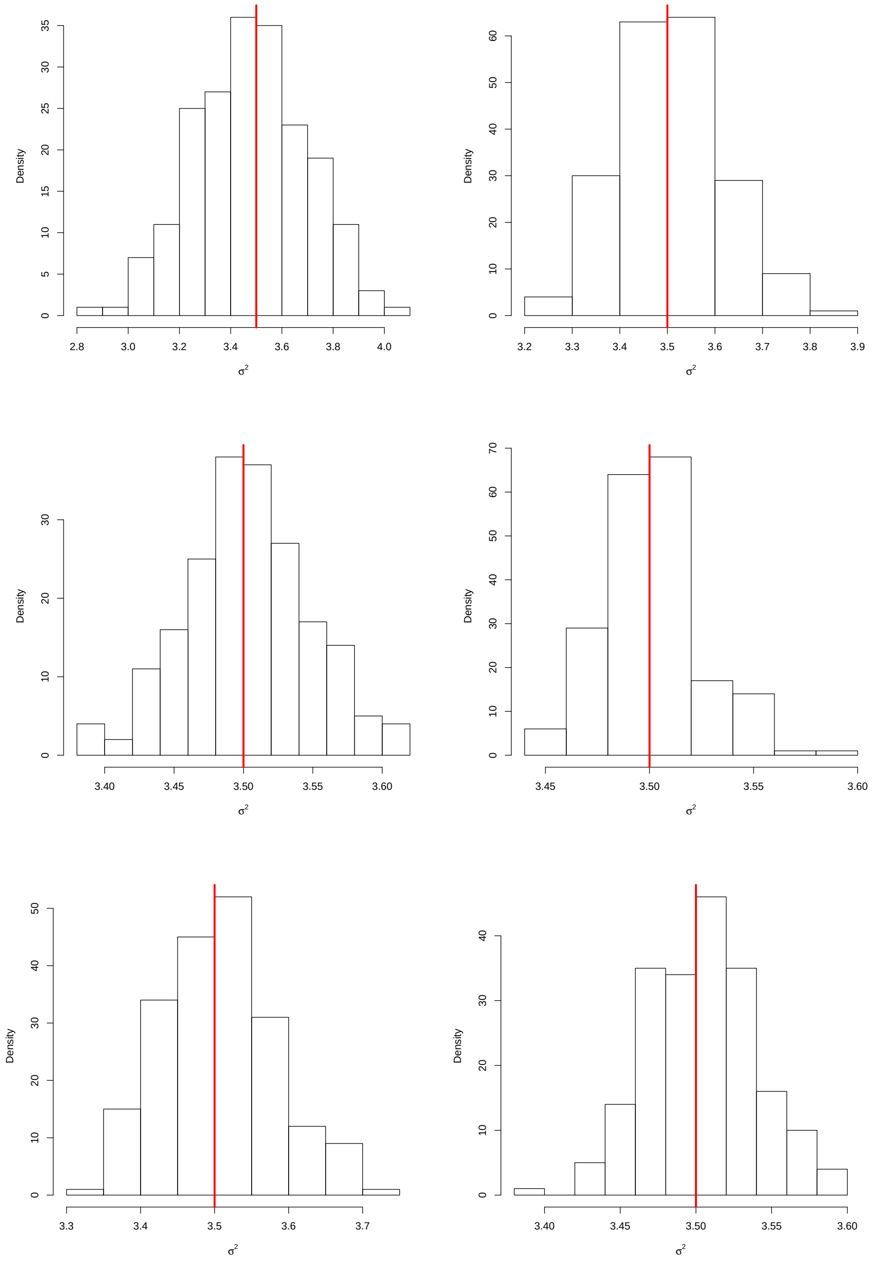


Figure 15: Case 3 ($\alpha_1$ *is much smaller than* $\alpha_2$ *and the* $M$*'s are balanced*): histogram of the 200 estimates of the variance of the white noise as in Figure 13.

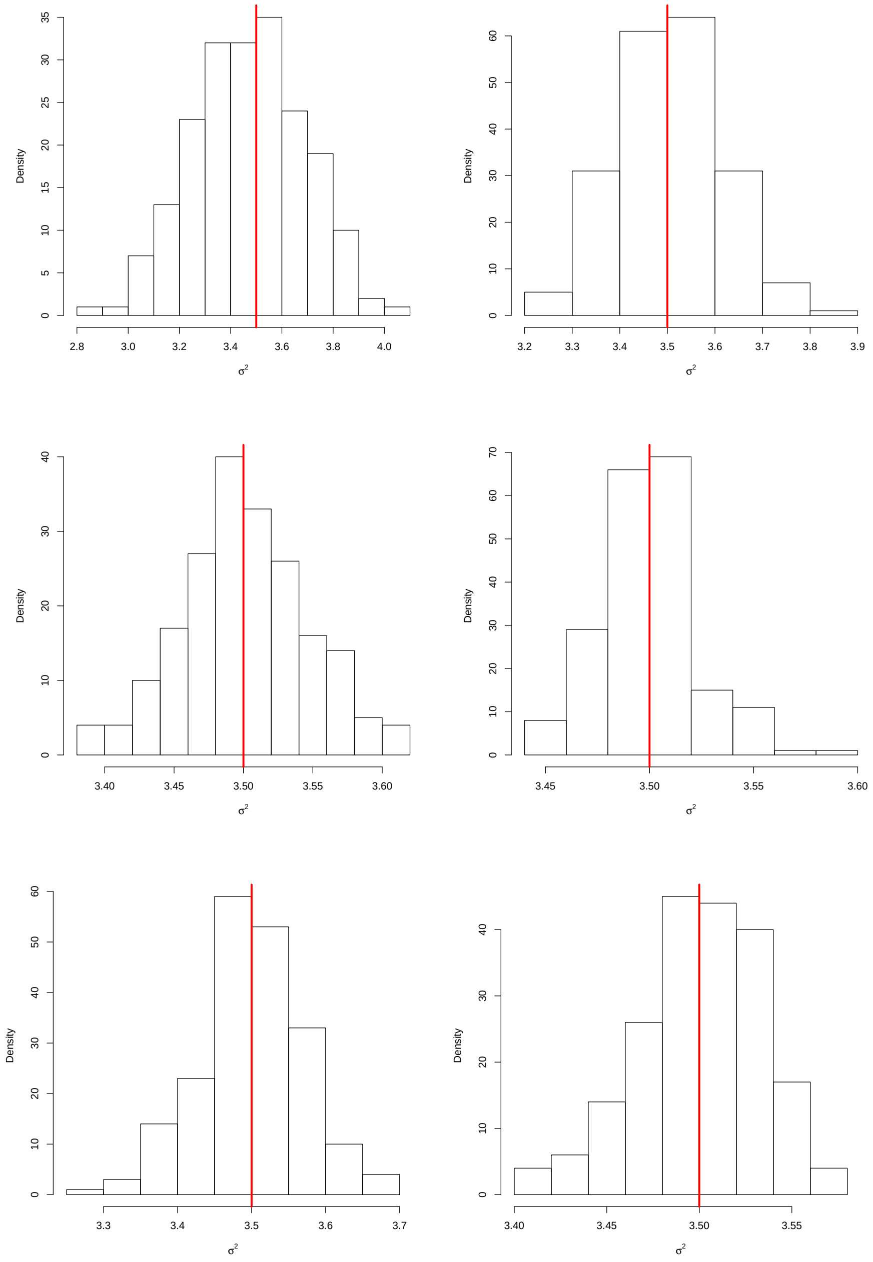


Figure 16: Case 4 ($\alpha_1$ *is much smaller than* $\alpha_2$ *and the* $M_1$*'s are much bigger than the* $M_2$*'s*): histogram of the 200 estimates of the variance of the white noise as in Figure 13.

| Case | $I$ | #R's | 1000×Var | 1000×Bias |
|---|---|---|---|---|
| 1<br>$\alpha_1 \approx \alpha_2$<br>balanced $M$'s | 5 | 1 | 47.96 | 42.43 |
| | 5 | 5 | 11.94 | -9.26 |
| | 5 | 30 | 2.09 | -3.37 |
| | 5 | 100 | **0.57** | **-1.72** |
| | 50 | 1 | 5.70 | -6.09 |
| | 50 | 5 | 1.29 | -4.35 |
| 2<br>$\alpha_1 \approx \alpha_2$<br>unbalanced $M$'s | 5 | 1 | 46.83 | 45.29 |
| | 5 | 5 | 11.76 | -9.04 |
| | 5 | 30 | 2.07 | -3.31 |
| | 5 | 100 | **0.58** | -1.69 |
| | 50 | 1 | 1.13 | **-0.18** |
| | 50 | 5 | 1.29 | -4.28 |
| 3<br>$\alpha_1 << \alpha_2$<br>balanced $M$'s | 5 | 1 | 48.17 | 27.63 |
| | 5 | 5 | 11.96 | -9.35 |
| | 5 | 30 | 2.10 | -3.35 |
| | 5 | 100 | **0.57** | **-1.58** |
| | 50 | 1 | 5.71 | -6.76 |
| | 50 | 5 | 1.31 | -4.06 |
| 4<br>$\alpha_1 << \alpha_2$<br>unbalanced $M$'s | 5 | 1 | 47.71 | 32.24 |
| | 5 | 5 | 11.81 | -6.64 |
| | 5 | 30 | 2.07 | -1.46 |
| | 5 | 100 | **0.57** | **0.23** |
| | 50 | 1 | 4.73 | -0.92 |
| | 50 | 5 | 1.30 | -2.18 |

Table 1: Empirical variance and bias of the 200 estimates of the variance of the white noise, $\sigma^2$, for Cases 1, 2, 3 and 4 considering $I = 5$ transformers with 1, 5, 30 and 100 replicates and $I = 50$ transformers with 1 and 5 replicates. The smallest values of variance and bias for each case are in bold font.

| Case | $I$ | #R's | $\sigma^2_{\gamma,1}$ % = 0 | $\sigma^2_{\gamma,1}$ 1000×Var | $\sigma^2_{\gamma,1}$ 1000×Bias | $\sigma^2_{\gamma,2}$ % = 0 | $\sigma^2_{\gamma,2}$ 1000×Var | $\sigma^2_{\gamma,2}$ 1000×Bias |
|---|---|---|---|---|---|---|---|---|
| 1 $\alpha_1 \approx \alpha_2$ balanced $M$'s | 5 | 1 | 84.0% | - | - | 16.0% | - | - |
| | 5 | 5 | 3.5% | - | - | 0% | 0.23 | 2.23 |
| | 5 | 30 | 0% | 0.03 | 1.23 | 0% | 0.03 | -1.01 |
| | 5 | 100 | 0% | **0.01** | 1.36 | 0% | **0.01** | -1.88 |
| | 50 | 1 | 0% | 0.07 | 5.42 | 0% | 0.08 | 5.49 |
| | 50 | 5 | 0% | **0.01** | **0.16** | 0% | 0.02 | **-0.90** |
| 2 $\alpha_1 \approx \alpha_2$ unbalanced $M$'s | 5 | 1 | 79.5% | - | - | 19.0% | - | - |
| | 5 | 5 | 7.0% | - | - | 20.5% | - | - |
| | 5 | 30 | 0% | 0.03 | 1.04 | 7% | - | - |
| | 5 | 100 | 0% | **0.01** | **0.56** | 0% | 0.54 | -7.63 |
| | 50 | 1 | 0% | 0.04 | 3.02 | 0% | 0.20 | 8.44 |
| | 50 | 5 | 0% | **0.01** | -0.79 | 0% | **0.04** | **0.27** |
| 3 $\alpha_1 << \alpha_2$ balanced $M$'s | 5 | 1 | 99.5% | - | - | 0.5% | - | - |
| | 5 | 5 | 79.5% | - | - | 0% | 7.41 | 76.90 |
| | 5 | 30 | 86.5% | - | - | 0% | 1.15 | -12.03 |
| | 5 | 100 | 94.5% | - | - | 0% | **0.40** | -19.86 |
| | 50 | 1 | 74.5% | - | - | 0% | 3.94 | 100.34 |
| | 50 | 5 | 54.0% | - | - | 0% | 0.94 | **-2.67** |
| 4 $\alpha_1 << \alpha_2$ unbalanced $M$'s | 5 | 1 | 99.5% | - | - | 3.5% | - | - |
| | 5 | 5 | 92.0% | - | - | 0% | 9.76 | 51.00 |
| | 5 | 30 | 99.0% | - | - | 0% | 1.40 | -31.38 |
| | 5 | 100 | 100% | - | - | 0% | **0.42** | -42.24 |
| | 50 | 1 | 65.0% | - | - | 0% | 3.74 | 87.46 |
| | 50 | 5 | 5.0% | - | - | 0% | 1.01 | **-9.48** |

Table 2: Percentage of the 200 estimates of $\sigma^2_{\gamma,1}$ and $\sigma^2_{\gamma,2}$ that are equal to zero along with the empirical variance and bias (only for the scenarios without zeros) for Cases 1, 2, 3 and 4 considering $I = 5$ transformers with 1, 5, 30 and 100 replicates and $I = 50$ transformers with 1 and 5 replicates. The smallest values of variance and bias for each case are in bold font.

| Transformer | $\widehat{M}_1$ | | | | | | | | | | | | | |
|---|---|---|---|---|---|---|---|---|---|---|---|---|---|---|
| | $I = 5$ | | | | | | | $I = 50$ | | | | | | |
| # 1 | 42 | 43 | 44 | [**45**] | 46 | 47 | 48 | 42 | 43 | 44 | [**45**] | 46 | 47 | 48 |
| 1 without replication | 0 | 6 | 34 | 96 | 57 | 6 | 1 | 0 | 11 | 54 | 95 | 38 | 2 | 0 |
| 3 without replication | 0 | 1 | 14 | 83 | 92 | 10 | 0 | 0 | 5 | 49 | 121 | 24 | 1 | 0 |
| 1 with 5 replications | 0 | 0 | 11 | 180 | 9 | 0 | 0 | 0 | 0 | 38 | 160 | 2 | 0 | 0 |
| 3 with 5 replications | 0 | 0 | 0 | 145 | 55 | 0 | 0 | 0 | 0 | 13 | 185 | 2 | 0 | 0 |
| # 2 | 27 | 28 | **29** | 30 | 31 | [32] | 33 | 27 | 28 | **29** | 30 | 31 | [32] | 33 |
| 1 without replication | 0 | 3 | 24 | 61 | 74 | 35 | 3 | 2 | 23 | 51 | 88 | 32 | 4 | 0 |
| 3 without replication | 0 | 1 | 7 | 37 | 97 | 55 | 3 | 0 | 31 | 75 | 74 | 19 | 1 | 0 |
| 1 with 5 replications | 0 | 0 | 0 | 63 | 135 | 2 | 0 | 0 | 0 | 51 | 137 | 12 | 0 | 0 |
| 3 with 5 replications | 0 | 0 | 0 | 25 | 161 | 14 | 0 | 0 | 4 | 95 | 101 | 0 | 0 | 0 |
| # 3 | 49 | 50 | [60] | **61** | 62 | 63 | 64 | 49 | 50 | [60] | **61** | 62 | 63 | 64 |
| 1 without replication | 0 | 7 | 173 | 20 | 0 | 0 | 0 | 0 | 9 | 79 | 84 | 26 | 1 | 0 |
| 3 without replication | 0 | 2 | 197 | 1 | 0 | 0 | 0 | 0 | 1 | 77 | 106 | 16 | 0 | 0 |
| 1 with 5 replications | 0 | 0 | 200 | 0 | 0 | 0 | 0 | 0 | 0 | 83 | 114 | 3 | 0 | 0 |
| 3 with 5 replications | 0 | 0 | 200 | 0 | 0 | 0 | 0 | 0 | 0 | 18 | 180 | 2 | 0 | 0 |
| # 4 | 23 | **24** | 25 | 26 | 27 | [28] | 29 | 20 | 22 | 23 | **24** | 25 | 26 | 27 |
| 1 without replication | 1 | 8 | 26 | 85 | 57 | 22 | 1 | 1 | 1 | 13 | 49 | 74 | 53 | 9 |
| 3 without replication | 0 | 2 | 17 | 68 | 89 | 24 | 0 | 0 | 3 | 12 | 90 | 65 | 25 | 5 |
| 1 with 5 replications | 0 | 0 | 2 | 144 | 54 | 0 | 0 | 0 | 0 | 0 | 24 | 137 | 39 | 0 |
| 3 with 5 replications | 0 | 0 | 3 | 116 | 80 | 1 | 0 | 0 | 0 | 0 | 59 | 138 | 3 | 0 |
| # 5 | 11 | **12** | 13 | 14 | 15 | [16] | 17 | 10 | 11 | **12** | 13 | 14 | 15 | [16] |
| 1 without replication | 0 | 0 | 11 | 47 | 106 | 35 | 1 | 1 | 18 | 65 | 78 | 29 | 9 | 0 |
| 3 without replication | 0 | 0 | 0 | 22 | 82 | 82 | 14 | 1 | 27 | 63 | 81 | 26 | 2 | 0 |
| 1 with 5 replications | 0 | 0 | 2 | 93 | 105 | 0 | 0 | 0 | 0 | 45 | 153 | 2 | 0 | 0 |
| 3 with 5 replications | 0 | 0 | 1 | 22 | 163 | 14 | 0 | 0 | 0 | 70 | 127 | 3 | 0 | 0 |

Table 3: Tables of the simulated distribution of $\hat{M}_1$, the estimated number of consumers of class $c = 1$ (residential), in transformers $i = 1, \ldots, 5$ for simulations with balanced $M$'s (Cases 1 and 3) and $I = 5$ (left column) and $I = 50$ (right column) transformers. In Case 1 $\alpha_1$ and $\alpha_2$ are of the same scale and in Case 3 $\alpha_1$ is much smaller than $\alpha_2$. In each table, the column heading contains different possible estimate values with the true value of $M_1$ in bold font and the reported value within brackets. Each of the remaining rows corresponds to a different simulation scenario. Each row contains the number of estimates of $M_1$ (out of the 200 estimates) that are equal to the associated column heading. Note that in transformer 1 the true and reported counts are both equal to 45. In transformers 4 and 5 with $I = 50$ none of the estimates was equal the reported count.

| Transformer | $\widehat{M}_1$ | | | | | | | | | | | |
|---|---|---|---|---|---|---|---|---|---|---|---|---|
| | $I = 5$ | | | | | | $I = 50$ | | | | | |
| # 1 | 64 | [65] | **66** | 67 | 68 | 69 | 64 | [65] | **66** | 67 | 68 | 69 |
| 2 without replication | 1 | 64 | 90 | 31 | 4 | 10 | 3 | 58 | 95 | 9 | 0 | 35 |
| 4 without replication | 0 | 25 | 159 | 16 | 0 | 0 | 1 | 55 | 133 | 11 | 0 | 0 |
| 2 with 5 replications | 0 | 26 | 161 | 13 | 0 | 0 | 0 | 33 | 162 | 0 | 0 | 5 |
| 4 with 5 replications | 0 | 2 | 198 | 0 | 0 | 0 | 0 | 7 | 193 | 0 | 0 | 0 |
| # 2 | 63 | 64 | **65** | [66] | 67 | 68 | 63 | 64 | **65** | [66] | 67 | 68 |
| 2 without replication | 0 | 5 | 63 | 109 | 21 | 2 | 0 | 4 | 36 | 130 | 28 | 2 |
| 4 without replication | 0 | 0 | 144 | 56 | 0 | 0 | 0 | 14 | 155 | 31 | 0 | 0 |
| 2 with 5 replications | 0 | 0 | 7 | 192 | 1 | 0 | 0 | 0 | 3 | 193 | 4 | 0 |
| 4 with 5 replications | 0 | 0 | 170 | 30 | 0 | 0 | 0 | 0 | 188 | 12 | 0 | 0 |
| # 3 | 66 | 67 | [68] | **69** | 70 | 71 | 66 | 67 | [68] | **69** | 70 | 71 |
| 2 without replication | 1 | 15 | 105 | 59 | 20 | 0 | 0 | 2 | 57 | 118 | 23 | 0 |
| 4 without replication | 0 | 0 | 111 | 89 | 0 | 0 | 0 | 0 | 47 | 149 | 4 | 0 |
| 2 with 5 replications | 0 | 0 | 93 | 107 | 0 | 0 | 0 | 0 | 14 | 186 | 0 | 0 |
| 4 with 5 replications | 0 | 0 | 129 | 71 | 0 | 0 | 0 | 0 | 3 | 197 | 0 | 0 |
| # 4 | 60 | 61 | **62** | [63] | 64 | 65 | 59 | 60 | 61 | **62** | [63] | 64 |
| 2 without replication | 0 | 0 | 20 | 133 | 45 | 2 | 0 | 0 | 10 | 42 | 118 | 30 |
| 4 without replication | 0 | 0 | 53 | 145 | 2 | 0 | 0 | 0 | 21 | 140 | 38 | 1 |
| 2 with 5 replications | 0 | 0 | 0 | 194 | 6 | 0 | 0 | 0 | 0 | 10 | 187 | 3 |
| 4 with 5 replications | 0 | 0 | 5 | 195 | 0 | 0 | 0 | 0 | 1 | 177 | 22 | 0 |
| # 5 | 69 | 70 | [71] | **72** | 73 | 74 | 69 | 70 | [71] | **72** | 73 | 74 |
| 2 without replication | 0 | 2 | 147 | 51 | 0 | 0 | 0 | 0 | 42 | 136 | 22 | 0 |
| 4 without replication | 0 | 0 | 200 | 0 | 0 | 0 | 0 | 0 | 52 | 147 | 1 | 0 |
| 2 with 5 replications | 0 | 0 | 178 | 22 | 0 | 0 | 0 | 0 | 6 | 193 | 1 | 0 |
| 4 with 5 replications | 0 | 0 | 200 | 0 | 0 | 0 | 0 | 0 | 4 | 196 | 0 | 0 |

Table 4: Tables of the simulated distribution of $\hat{M}_1$, the estimated number of consumers of class $c = 1$ (residential), in transformers $i = 1, \ldots, 5$ for simulations with unbalanced $M$'s (Cases 2 and 4) and $I = 5$ (left column) and $I = 50$ (right column) transformers as in Table 3. In Case 2 $\alpha_1$ and $\alpha_2$ are of the same scale and in Case 4 $\alpha_1$ is much smaller than $\alpha_2$.
